# Supplementary material for: A lattice on Dyck paths close to the Tamari lattice
Source: arXiv:2309.00426 source file (2025-05-13)
Supplement: Supplementary file 1 [file appendix.tex]

\appendix\section{Appendix}\label{sec:appendix}

%%% Local Variables:
%%% mode: latex
%%% TeX-master:"../../paper_discrete.tex"
%%% End:
